# Supplementary material for: Reading Strategies for Graph Visualizations that Wrap Around in Torus Topology
Source: arXiv:2303.17066 source file (2023-04-26)
Supplement: Supplementary file 1 [file appendix.tex]

\section{Gallery}
\label{sec:appendix}
This section describes supplementary materials. 
This includes other stimuli of shortest path tasks that involve different wrapping directions of the unique shortest path, as well as link counting tasks.

An evaluation of space utilization of \tfullcontext{} is illustrated in~\autoref{fig:aoi-percentage-time}.
Results indicate that for \tfullcontext{}, the center cell is used most often, while corner cells are still necessary (c). Gaze allocation in different levels of replicated context (d) indicates that space utilization of \tfullcontext{} could be more efficient by discarding the Outer3 AOI. 
\begin{figure}
    \centering
    
     \includegraphics[width=1.0\textwidth]{figures/overview_reading_strategy-supple.png}
    
    \Description[]{}
    \caption[]{
    Density maps of time-aggregated fixation distributions for \tshortestpath{}, overlaid in the original image of four network layouts of medium-sized stimuli. Higher saturation indicates denser fixation distribution over regions of the image. The subcaption below each image indicates wrapping setting regarding the wrapping directions of the unique shortest path. The radius of the light blue dots indicate the fixation duration. \label{fig:densitymaps_shortest_path}
    }
\end{figure}

\begin{figure}
    \centering
    
     \includegraphics[width=1.0\textwidth]{figures/overview_reading_strategy-large-supple.png}
    
    \Description[]{}
    \caption[]{
    Density maps of time-aggregated fixation distributions for \tshortestpath{}, overlaid in the original image of four network layouts of large-sized stimuli. Higher saturation indicates denser fixation distribution over regions of the image. The subcaption below each image indicates wrapping setting regarding the wrapping directions of the unique shortest path. The radius of the light blue dots indicate the fixation duration. \label{fig:overview_reading_strategy-large-supple}
    }
\end{figure}

\begin{figure}
    \centering
    
     \includegraphics[width=1.0\textwidth]{figures/density_maps_linkcount.png}
    
    \Description[]{}
    \caption[]{Density maps and visual fixation sequence (encoded in dots with increasing saturation of colours showing temporal gaze sequence) of time aggregated 13 participants' gaze data, overlaid in stimuli images; Each stimuli image shows an example where the participant were asked to count the total number of links in the network diagram. Some links are wrapped around in top-bottom or left-right wrapping; Others are without wrapping; The density maps depict overall user attention distribution in central or boundary region of the network diagram. \label{fig:densitymaps_linkcount}
    }
\end{figure}

\begin{figure}
    \centering
     \subfigure[three-by-three-tiled AOIs]{
    \includegraphics[width=0.4\columnwidth]{figures/FC_3-by-3-AOIs_utilisation.jpg}
    }
    \subfigure[Inner to outer tiled AOIs with increasing distance from the center]{
    \includegraphics[width=0.4\columnwidth]{figures/FC_in-to-out-AOIs_utilisation.jpg}
    }
    \subfigure[AOI percentage time of three-by-three-tiled AOIs]{
    \includegraphics[width=0.3\columnwidth]{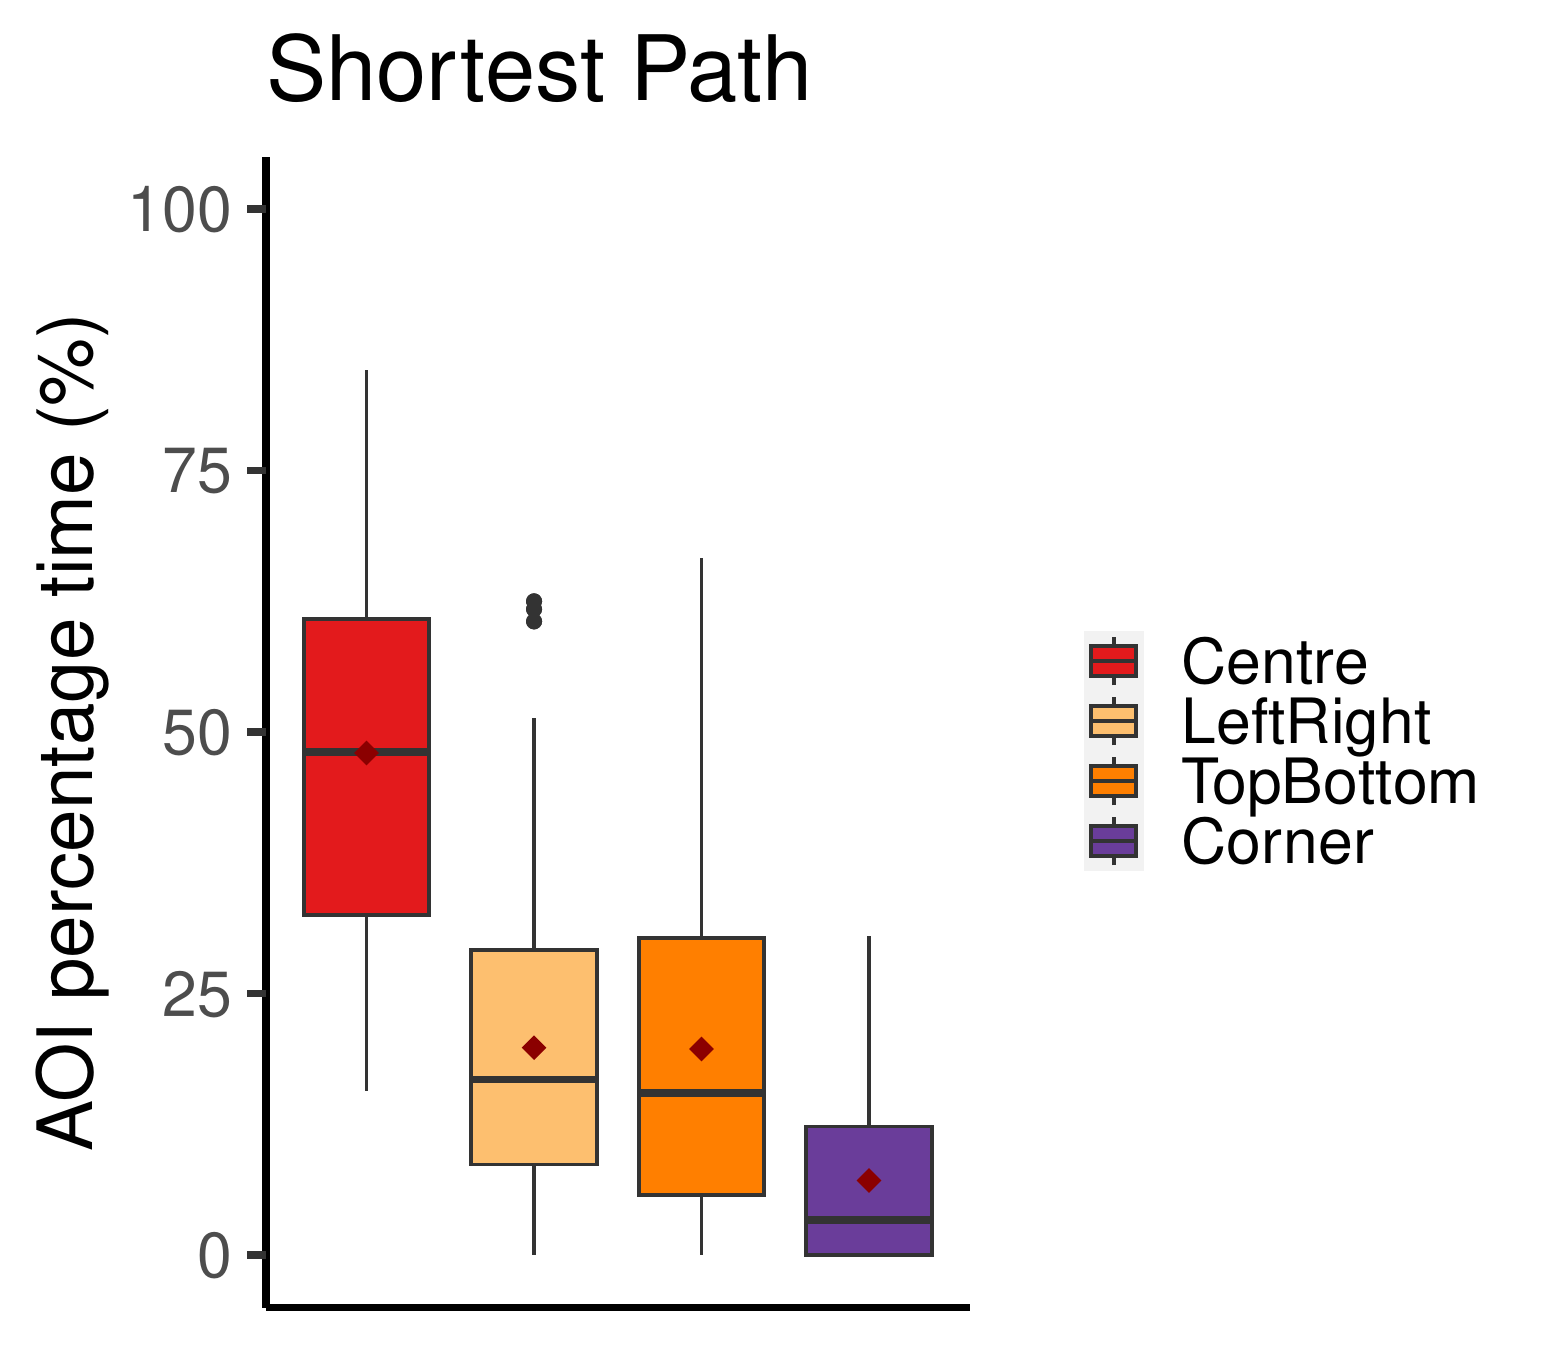}
    }
    \subfigure[AOI percentage time of AOIs from inner to outer regions]{
    \includegraphics[width=0.3\columnwidth]{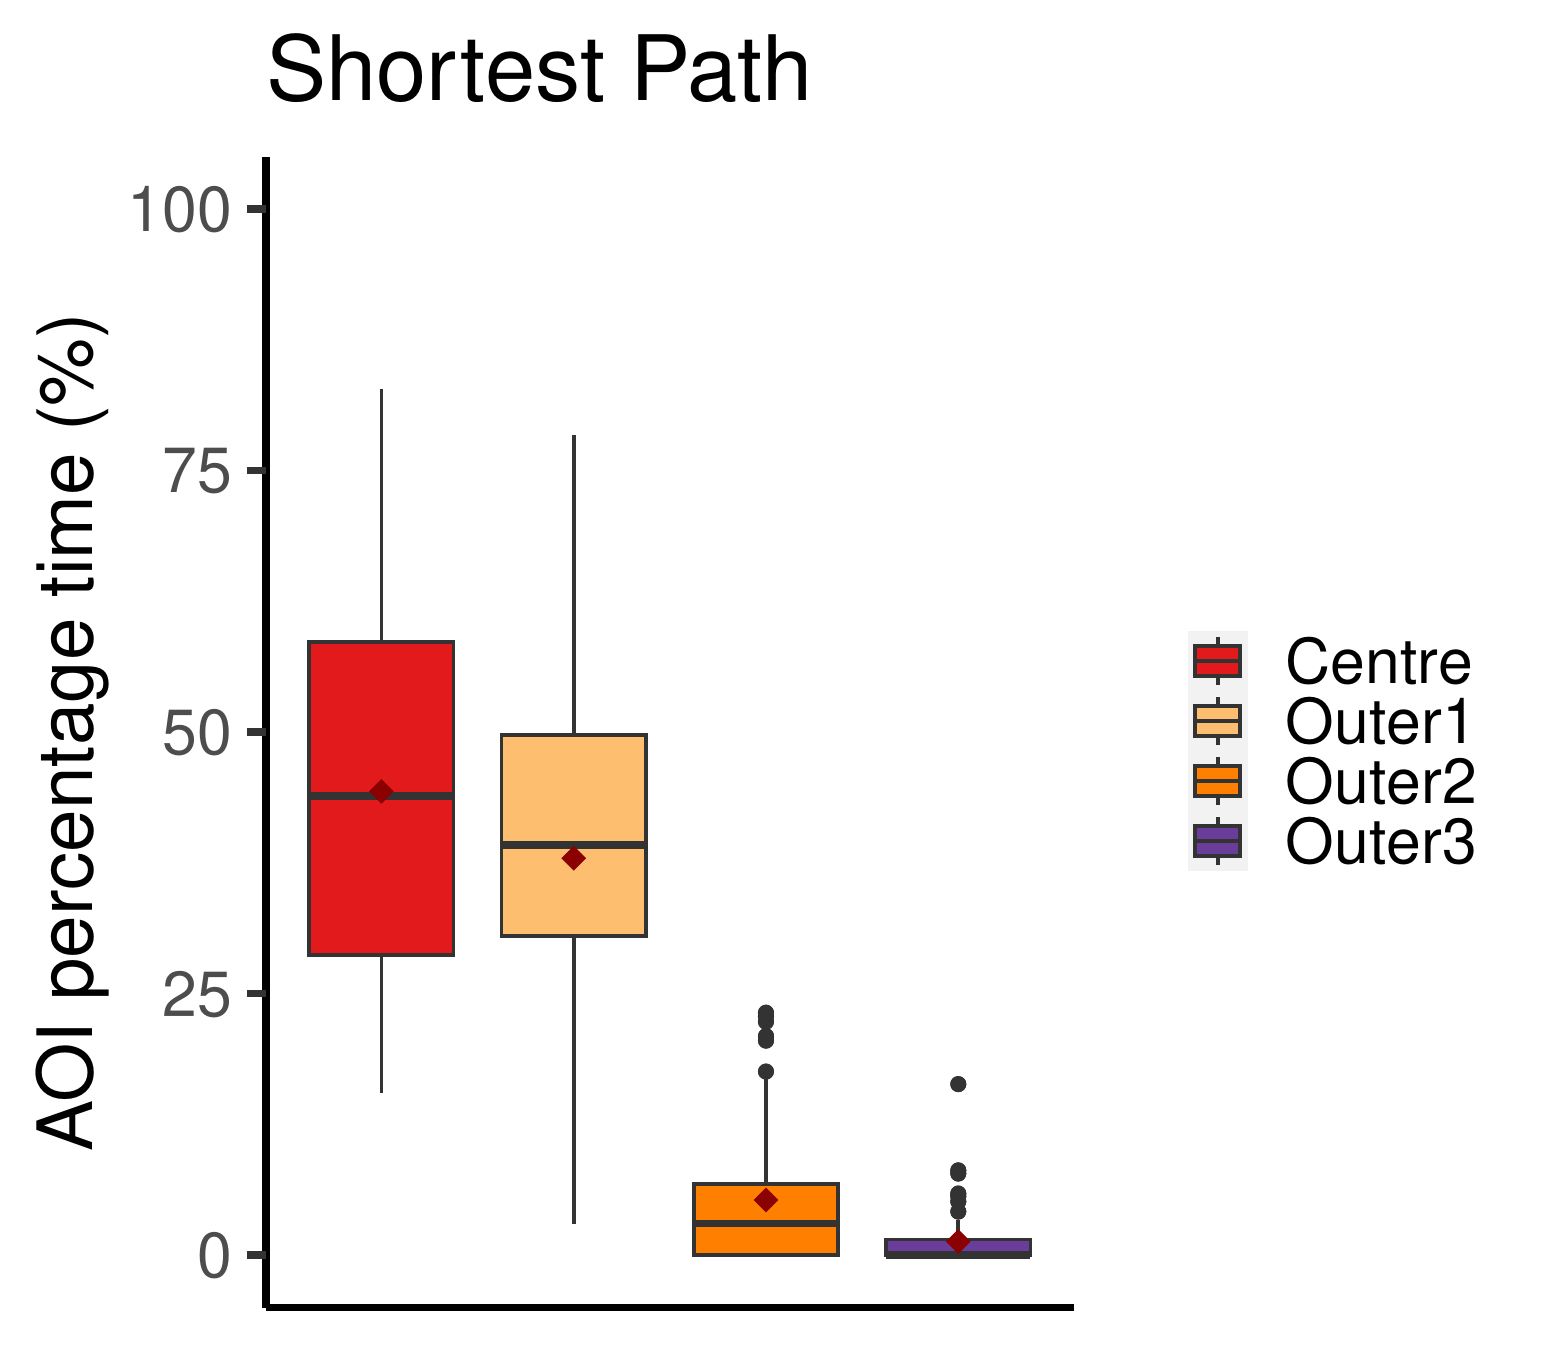}
    }
    \Description[]{Box plot and spatial view of fixation of AOI percentage time where AOIs are defined by tiles (a-b) and by increasing distance from the center cell (c-d), across medium and large stimuli of shortest path tasks}
    \caption[]{Box plot of results of all the medium-and-large-sized graphs of participants' relative fixation duration (AOI percentage time) out of total time spent performing an experimental trial, where AOIs are defined as tiles (a-c) and by increasing distance from the center cell (b-d), across all participants performing medium and large stimuli of shortest path tasks; the corresponding spatial view of aggregated fixations are shown in (a) and (b), respectively. 
    Dotted lines indicate significant differences.    
    }
    \label{fig:aoi-percentage-time}
    % \vspace{-1em}
\end{figure}
